# Supplementary material for: Review4Repair: Code Review Aided Automatic Program Repairing
Source: arXiv:2010.01544 source file (2020-10-06)
Supplement: Supplementary file 1 [file Appendix.tex]

\begin{figure}[ht]
\centering
\includegraphics[width=\linewidth]{images/dataset_with_table.eps}
\caption{Code and Review Count per Project}
\label{fig:dataset}
\end{figure}
